# Supplementary material for: Benchmarking Hydrogen-Helium Mixtures with QMC: Energetics, Pressures, and Forces
Source: arXiv:1508.05118 source file (2015-08-20)
Supplement: Supplementary file 1 [file supplemental_info.pdf]

# I. THEORY

## A. Finite Size Effects

Our QMC and DFT calculations were performed on snapshots of disordered liquid configurations at T=7000K in periodic boundary conditions. Each snapshot then serves as the starting point for independent ground-state calculations using clamped nuclei. Since the DFT calculations were converged with respect to Monkhorst-Pack k-point mesh, the problem is equivalent to solving the electronic structure problem for a crystal in the thermodynamic limit, whose unit cell is given by the snapshot arrangement of atoms. We need to compensate for the one and two-body finite-size stemming from the QMC calculations in this setting.

We will focus on how the total energy per electron, $E_N = \langle \hat{H} \rangle / N_e$ approaches the thermodynamic limit. $N_e$ is the number of electrons. Specifically, we will look at how the kinetic energy $T_N = \langle \hat{T} \rangle / N_e$ and potential energy $V_N = \langle \hat{V} \rangle / N_e$ differ from the thermodynamic limit.

Because we will need it later, the fourier transform of the particle density of species $\alpha$ is given by $\rho^{\alpha}_{\mathbf{G}} = \sum_{j_\alpha} e^{i\mathbf{G}\cdot\mathbf{r}_{j_\alpha}}$. Here, $\mathbf{r}_{j_\alpha}$ denotes the 3D coordinate vector of particle $j$ of species $\alpha$.

### 1. One-Body

It is well known that one of the biggest one-particle finite size errors that emerge in QMC calculations are "shell-effects", which stem from the fact that single-particle occupations can only be discrete. This is drastically reduced through the use of twist-averaging[1]. In our work, we use "canonical twist averaging", whereby the particle number is fixed at all sampled twists, and occupations are determined by the usual energy criterion within DFT.

Through consistent occupations above the fermi-surface, canonical twist-averaging introduces a small positive bias to the total energy (<1mHa/N). We estimate and correct for this effect, we consider an auxiliary single particle theory for our system, given by:

$$\left(-\frac{\hbar^2}{2m}\nabla^2 + v_{eff}(\mathbf{r})\right)\phi_i(\mathbf{r}) = \epsilon_i \phi_i(\mathbf{r}) \tag{1}$$

Here, we chosen to be $v_{eff}(\mathbf{r})$ as calculated from a self-consistent PBE calculation within a 64 electron unit cell on a 7x7x7 MP grid. As an initial approximation to our fermi-surface, we calculated the single particle energy (summing eigenvalues) by doubly occupying all orbitals in a 7x7x7 is equivalent to a 21,952 electron supercell. Then, for the 64 electron unit cell, we computed the single-particle energy for each k-point by again doubly occupying the orbitals at a specific k-point. After averaging the single-particle energy over all k-points, we calculated the difference between the 21,952 electron and the twist-averaged 64 electron single-particle energies. For the highest densities and hydrogen fractions, this effect was found to be as large as 0.7mHa/N, though it decreased with increasing helium concentrations and decreasing density.

Other residual one-body errors are due to the fact that $\rho^{e}_{\mathbf{G},N}$ has not converged to the thermodynamic limit for fixed $\mathbf{G}$. This is a higher order effect, and we do not try to correct it at the QMC level. Though we can attempt to gauge the magnitude again by DFT, we ignore the effect in this discussion.

### 2. Two-Body

The next largest source of finite size errors stems from the electron-electron interaction terms. Following the Chiesa scheme[2], we run under the assumption that the largest contribution stems from an "integration error". Specifically, we assume that the structure factor $S_N(\mathbf{k}) = \langle \rho_{-\mathbf{k}} \rho_{\mathbf{k}} \rangle / N$ is close to the thermodynamic limiting values at k-points commensurate with the simulation cell.

There is a question regarding which structure factor to use, as the general potential energy contains terms like $\rho^{\alpha}_{-\mathbf{k}}\rho^{\beta}_{\mathbf{k}}$, with each species having a different number of particles. From the problem specifications mentioned at the beginning of this subsection, the following statements are true regarding finite size effects in our systems:

1. **There are no finite size effects stemming from the ion-ion terms**: This is a direct consequence of the clamped nuclei condition.

2. **The only finite size effects stemming from the electron-ion terms are from the electron density**: Again, since we are using clamped nuclei all $\rho^{\alpha}_{\mathbf{G}}$ and $e^{i\mathbf{G}\cdot\mathbf{r}_{i_\alpha}}$ terms are **constants**. This means that the only term that can change as one progresses to the thermodynamic limit is the average electron density $\langle \rho^{e}_{\mathbf{G}} \rangle$.

3. **The dominant finite-size effect stemming from the electron-electron interaction is due to long-ranged electron *fluctuations***: Write $\rho^e_{\mathbf{G}} = \langle \rho^e_{\mathbf{G}} \rangle + \delta\rho^e_{\mathbf{G}}$. This yields $\langle \rho^e_{-\mathbf{G}} \rho^e_{\mathbf{G}} \rangle = \langle \rho^e_{-\mathbf{G}} \rangle \langle \rho^e_{\mathbf{G}} \rangle + \langle \delta\rho^e_{-\mathbf{G}} \delta\rho^e_{\mathbf{G}} \rangle$. Assuming that the average electron density is reasonably converged, the main contributor to the finite size effects will be $\langle \delta\rho^e_{-\mathbf{G}} \delta\rho^e_{\mathbf{G}} \rangle$.

The last point is particularly important: at k-points incommensurate with the unit cell, the electron-electron structure factor and the "fluctuation" structure factor will equal eachother. This is because the static electronic charge density $\langle \rho^e_{\mathbf{G}} \rangle = 0$ at these k-points. This would not cause problems in a large enough supercell calculation, assuming one only fits the first few k-shells, but the distinction is important when we attempt to fit the structure factor in small supercells. We stress that the correct structure factor to use in these cases is the "fluctuation" structure factor $S_{\delta\delta}(\mathbf{k}) = \langle \delta\rho^e_{-\mathbf{G}} \delta\rho^e_{\mathbf{G}} \rangle / N_e$.

### B. QMC Force Estimation

By the Hellman-Feynman theorem,

$$\mathbf{F}_{p_\alpha} = \frac{\langle \Psi | - \nabla_{p_\alpha} \hat{H} | \Psi \rangle}{\langle \Psi | \Psi \rangle} \tag{2}$$

Assuming clamped nuclei, the kinetic energy in our Hamiltonian $\hat{H}$ has no dependence on the ionic coordinates. Additionally, the ion-ion force contributions do not depend on the electronic coordinates, so these can be evaluated exactly.

It is useful to decompose the total force on ion $p$ of species $\alpha$ as $\mathbf{F}_{p_\alpha} = \mathbf{F}^I_{p_\alpha} + \mathbf{F}^e_{p_\alpha}$. The ionic contribution to the force, $\mathbf{F}^I_{p_\alpha}$, is computed in one shot at the beginning of the simulation. The electron-ion contribution is given by

$$\mathbf{F}^e_{p_\alpha} = \langle \Psi | \sum_{i_e} \frac{d}{dr} \sigma^{\alpha e}(|\mathbf{r}_{i_e} - \mathbf{r}_{p_\alpha}|) \frac{\mathbf{r}_{i_e} - \mathbf{r}_{p_\alpha}}{|\mathbf{r}_{i_e} - \mathbf{r}_{p_\alpha}|} + \sum_{\mathbf{G} \neq 0} \Lambda^{\alpha\beta}_{\mathbf{G}} \Im \left( e^{i\mathbf{G}\cdot\mathbf{r}_{p_\alpha}} \rho^e_{\mathbf{G}} \right) \mathbf{G} | \Psi \rangle / \langle \Psi | \Psi \rangle \tag{3}$$

Here, $\sigma^{\alpha e}(r)$ is the short-ranged radial potential coming from the optimized breakup of the coulomb potential, whereas $\Lambda_{\mathbf{G}}$ is the fourier component of the long-range part. The reciprocal space sum is smooth and non-divergent, and so has a finite variance. The magnitude of the short-range real space force, on the other hand, has a $1/r^2$ divergence as $r \to 0$, which means that the bare Hellman-Feynman estimator will have infinite variance. The solution to this problem is to use the Chiesa, Ceperley, Zhang scheme[3]. Though the s-wave filtering technique was developed for a bare coulomb potential (in open boundary conditions), we note the that derivation is general as long as the radially symmetric potential is continuous. Consider the expression for the total force on an ion located at the origin.

$$\mathbf{F} = \int d^3\mathbf{r} \rho(\mathbf{r}) h(r) \frac{\mathbf{r}}{r} \tag{4}$$

In the original derivation, $h(r) = Z/r^2$. In our case, $h(r) = \frac{d}{dr}\sigma(r) = Zw(r)/r^2$. To recover the short-ranged behavior of the electron-ion coulomb force term, $w(r) \to 1$ as $r \to 0$, and $w(r) \to r^3$ as $r \to r_c$. The latter condition stems from the fact that the short-ranged force magnitude should be constructed to go to zero outside a radius of $r_c$. Given these conditions, the arguments for the force density $f_z(r) \propto r$ as $r \to 0$ by the constraint that $\rho(r)$ be a physically reasonable density still holds. The reader is invited to verify that the derivation of the filtering function $g(r)$ in this paper remains unchanged with the substitution $Z/r^2 \to Zw(r)/r^2$. Thus, we can apply the Chiesa filtering scheme without modification to the short-range force terms to fix the divergence. Taking the operator between $\langle \Psi | \ldots | \Psi \rangle$ in Eq. I B and applying the Chiesa correction yields the following finite-variance operator $\hat{\mathbf{F}}^e_{p_\alpha}$:

$$\hat{\mathbf{F}}^e_{p_\alpha} = \sum_{i_e} g(|\mathbf{r}_{i_e} - \mathbf{r}_{p_\alpha}|) \frac{d}{dr} \sigma^{\alpha e}(|\mathbf{r}_{i_e} - \mathbf{r}_{p_\alpha}|) \frac{\mathbf{r}_{i_e} - \mathbf{r}_{p_\alpha}}{|\mathbf{r}_{i_e} - \mathbf{r}_{p_\alpha}|} + \sum_{\mathbf{G} \neq 0} \Lambda^{\alpha\beta}_{\mathbf{G}} \Im \left( e^{i\mathbf{G}\cdot\mathbf{r}_{p_\alpha}} \rho^e_{\mathbf{G}} \right) \mathbf{G} \tag{5}$$

From the original paper[3], $g(r) = \theta(\mathcal{R} - r) \sum_{k=1}^{M} c_k r^{k+m}$, where $c_k$ is given by $\mathbf{c} = \mathbf{S}^{-1}\mathbf{h}$. $\mathcal{R}$ is a real-space cutoff, and $M$ specifies the degree of the smoothing polynomial. $\mathbf{S}$ and $\mathbf{h}$ are given by:

$$S_{kj} = \frac{\mathcal{R}^{m+k+j+1}}{m+k+j+1} \tag{6}$$

$$h_j = \frac{\mathcal{R}^{j+1}}{j+1} \tag{7}$$

| | Finite Diff | Chiesa | $\Delta F$ |
|---|---|---|---|
| $F_x^e$ | -0.3260(27) | -0.3244(16) | -0.0016(31) |
| $F_y^e$ | 0.0997(27) | 0.0953(24) | 0.0044(34) |
| $F_z^e$ | 0.2840(28) | 0.2832(18) | 0.0008(33) |

TABLE I: VMC Electron-ion force $\mathbf{F}^e$ computed using the Chiesa-Ceperley-Zhang estimator and finite-differencing of local energy. The two agree to within the somewhat large error bars.

## II. TESTS

### A. Test of Force Estimator

In this section, we perform a finite difference test on an arbitrary H ion in a disordered system in periodic boundary conditions. This provides a check for both the optimized breakup routines and applying the Chiesa correction scheme in periodic boundary conditions.

Our trial system will be a snapshot from a path-integral molecular dynamics simulation of pure liquid H at T=1000K and $r_s = 1.60$. After choosing an atom, we calculated the three force components on this atom through two-point forward finite difference formulae. The energy differences between the trial displacements and our reference configuration were done simultaneously with VMC correlated sampling. Our step size was $h = 0.001a_0$. For the reference configuration we performed a VMC simulation to accumulate the Chiesa-Ceperley-Zhang estimator. We used $\mathcal{R} = 1.0a_0$, $M = 3$.

In Table I, we compute just the electron-ion contribution to the force $\mathbf{F}^e$ on a single hydrogen atom in our bulk snapshot using both the Chiesa-Ceperley-Zhang estimator and finite differencing (all at the VMC level). The maximum deviation of the Chiesa estimator from the finite difference results is 4.4mHa/$a_0$, which is well within error bars. This indicates that our procedure of performing the s-wave filtering directly on the short-ranged force components is correct.

We performed extensive studies of the biases associated with the choice of $\mathcal{R}$ and $M$, as well as the sensitivity of the extrapolated force estimates to the choice of trial wavefunction (we tested Slater-Jastrow and Slater-Jastrow with backflow wavefunctions). We find that our choice of $\mathcal{R} = 1.0$, $M = 3$, and the use of Slater-Jastrow wavefunctions produces force estimates that are statistically indistinguishable from force estimates based on smaller $\mathcal{R}$, larger $M$, or based on backflow wavefunctions.

Based on the finite differencing results and comparisons with more converged parameters, we expect the systematic force errors on the hydrogen atoms to be less than 2mHa/bohr (probably smaller), but indistinguishable from the error bars.

### B. Finite Size Effects

In this section, we describe and test the finite size correction scheme used in this manuscript. To establish a baseline, we performed 1/N extrapolations on a sample configuration with the following parameters: $r_s = 1.10$, $N_e = 64$, $N_H = 56$, and $N_{He} = 4$.

For the single-particle orbitals, we used plane-wave orbitals taken from PWSCF using the PBE functional. The plane-wave cutoff was $200Ry$. Orbitals were obtained on a 4x4x4 MP grid with an offset. We used all-electron pseudopotentials to smooth the 1/r divergence for both H and He. Troullier-Martin pseudopotentials[4] were generated with the PBE functional in the OPIUM code. The real space cutoff for both pseudopotentials was $0.37a_0$.

Single Slater-Jastrow wavefunctions without backflow are used for all subsequent calculations. The supercell is comprised of a 2x2x2 tiling of the unit cell, so we will refer to this cell often as the $N_e = 512$ cell. Twist averaging was done for all subsequent calculations. 4x4x4 MP grid with offset was used for the $N_e = 64$ cell, and 2x2x2 MP grid with offset was used for the $N_e = 512$ cell.

All energies are in $Ha/N_e$ and everything else should be in atomic units unless otherwise specified.

#### *1. Wavefunction #1*

This is representative of all the calculations done in our H+He study. The trial wavefunction is of the single Slater-Jastrow type. Jastrow factors are all short-ranged fully optimizable cubic b-splines. The same types of Jastrows are used in the $N_e = 512$ supercell, but the real space cutoffs are increased to span the simulation cell. We summarize the Jastrows used in the $N_e = 64$ cell in the Table II.

| Name | Type | Interaction | Function | $r_{cut}$ | Cusp | $N_{knots}$ | Optimizable |
|---|---|---|---|---|---|---|---|
| J2 | two-body | e-e (opposite spin) | b-spline | 3.546 | Yes | 10 | Yes |
| | two-body | e-e (like spin) | b-spline | 3.546 | Yes | 10 | Yes |
| J1L | one-body | e-H | b-spline | 3.546 | No | 8 | Yes |
| | one-body | e-He | b-spline | 3.546 | No | 8 | Yes |
| J1S | one-body | e-H | b-spline | 1.000 | Yes | 8 | Yes |
| | one-body | e-He | b-spline | 1.000 | Yes | 8 | Yes |

TABLE II: Summary of the Jastrow factors included in the trial wavefunction.

| Method | $N$ | $E$ | $\sigma^2_{E_L}$ | $V$ | $T$ | $V_{ee}$ | $V_{ei}$ |
|---|---|---|---|---|---|---|---|
| VMC | 64 | -0.534956(3) | 0.0371(2) | -1.70037(6) | 1.16541(6) | -0.477571(8) | -0.43699(7) |
| DMC | 64 | -0.538287(6) | – | -1.70513(5) | 1.16684(5) | -0.47973(2) | -0.43958(5) |
| EXTR | 64 | – | – | -1.7098(1) | 1.1682(1) | -0.48190(4) | -0.4421(1) |
| VMC | 512 | -0.524915(3) | 0.056(2) | -1.66134(6) | 1.13642(6) | -0.472809(9) | -0.40272(6) |
| DMC | 512 | -0.53184(1) | – | -1.68286(8) | 1.15102(8) | -0.47503(3) | -0.42201(8) |
| EXTR | 512 | – | – | -1.7043(2) | 1.1656(2) | -0.47726(6) | -0.4413(2) |

TABLE III: In this table, we compare the VMC, DMC, and EXTR(apolated) estimates for all components of the energy (excluding fixed ion-ion contribution) for wavefunction #1. All units are in Ha/N, where N is the number of electrons. No single particle effects beyond twist averaging are included.

Simulation parameters for $N_e = 64$ cell: For the VMC simulation, we used a time step of $\tau = 0.5$ with 512 walkers, with an accept probability of 0.669. For the DMC simulation, we used a time step of $\tau = 0.01 Ha^{-1}$ with 512 walkers, which gave an accept probability of 0.996.

Simulation parameters for $N_e = 512$ cell: For the VMC simulation, we used a time step of $\tau = 0.5$ with 1024 walkers, with an accept probability of 0.669. For the DMC simulation, we used a time step of $\tau = 0.01 Ha^{-1}$ with 1024 walkers, which gave an accept probability of 0.996.

### 2. *Wavefunction #2*

In addition to all the Jastrow terms appearing in wavefunction #1, we have included a k-space jastrow of the form:

$$J_2 = \frac{1}{\Omega} \sum_{\mathbf{G} \neq \mathbf{0}} a_{\mathbf{G}} \rho_{\mathbf{G}} \rho_{-\mathbf{G}} \tag{8}$$

For the k-space Jastrow, the sum was truncated at 7 k-vector shells. Both the unit cell and supercell used this form of wavefunction, and all k-space and real-space parameters were simultaneously (but independently) optimized in both cells.

In the unit cell, the VMC simulation had a time step of $\tau = 0.1 Ha^{-1}$, which gave an accept ratio of 0.926. For the reptation Monte Carlo (RMC) simulations, we used a projection time of $\beta = 5.16$ and two time steps: $\tau = 0.0075 Ha^{-1}$ (accept ratio 0.995) and $\tau = 0.00375 Ha^{-1}$ (accept ratio of 0.9974). We linearly extrapolated all mixed and pure estimates to $\tau = 0$.

Supercell: For the VMC a time step of $\tau = 0.2 Ha^{-1}$ was used, which gave an acceptance ratio of 0.86. For the RMC, we used a time step of $\tau = 0.0075$ and a projection time of $\beta = 4.0 Ha^{-1}$, which gave an acceptance ratio of 0.982.

It is worth noting in Table III that the extrapolated estimates of the potential energy based on wavefunction #1 are statistically indistinguishable from the pure RMC estimates based on wavefunction #2. Additionally, further checks have shown the same to be true of the structure factor. This strongly suggests that we can use extrapolated estimates based on wavefunction #1 to obtain accurate finite size corrections (the details of which are given in a later section).

## C. Finite Size Corrections

### 1. *KZK*

We performed the Kwee, Zhang, Krakauer[5] LDA based total energy finite size correction for this system. For each k-point used in the QMC twist averaging, we computed the KZK energy at all k-points used in twist-averaging for the

| Method | $N$ | $E$ | $\sigma^2_{E_L}$ | $V$ | $T$ | $V_{ee}$ | $V_{ei}$ |
|---|---|---|---|---|---|---|---|
| VMC | 64 | -0.536239(3) | 0.0273(2) | -1.7154(4) | 1.1792(4) | -0.47965(1) | -0.44999(4) |
| RMC | 64 | -0.53827(1) | – | -1.7073(1) | 1.1690(1) | -0.48030(5) | -0.44110(1) |
| EXTR | 64 | – | – | -1.6991(1) | 1.1588(1) | -0.48095(5) | -0.4323(1) |
| PURE | 64 | – | – | -1.7108(2) | 1.1726(2) | -0.48159(7) | -0.4434(2) |
| VMC | 512 | -0.52340(1) | 0.049(6) | -1.6814(1) | 1.1580(1) | -0.45538(3) | -0.4402(1) |
| RMC | 512 | -0.53172(2) | – | -1.6935(1) | 1.1619(1) | -0.46760(6) | -0.4401(1) |
| EXTR | 512 | – | – | -1.7056(3) | 1.1657(3) | -0.4798(1) | -0.4400(3) |
| PURE | 512 | – | – | -1.7059(4) | 1.1732(4) | -0.4760(1) | -0.4430(4) |

TABLE IV: In this table, we compare the VMC, RMC (mixed estimator), EXTR(apolated), and PURE (directly from RMC) estimates for all components of the energy (excluding fixed ion-ion contribution) for wavefunction #2. All units are in Ha/N, where N is the number of electrons. No single particle effects beyond twist averaging are included.

$N_e = 64$ electron system. Averaging over all twists, we obtained $\Delta E_N = 6.82$ mHa/N for the total energy correction.

### *2. MPC*

For all H+He runs, we accumulated the MPC[6,7] estimator of the infinite-system electron-electron energy. The correction is obtained by $\Delta V_{ee} = \langle V_{MPC}\rangle - \langle V_{ee}\rangle$. $V_{ee}$ is the average electron-electron energy for the $N_e = 64$ system. The results of this are tabulated in the following section.

### *3. Chiesa*

For the potential energy correction, we calculated the full $S_{\delta\delta}(\mathbf{k})$ fluctuation structure factor (see section X) for $\mathbf{k}$ vectors commensurate with the unit cell. This was done using both VMC and DMC. Using the extrapolated estimate of the fluctuation structure factor, $S^{EXT}_{\delta\delta}(\mathbf{k}) = 2S^{DMC}_{\delta\delta}(\mathbf{k}) - S^{VMC}_{\delta\delta}(\mathbf{k})$, we spherically averaged the full $S^{EXT}_{\delta\delta}(\mathbf{k})$, performed a 1D cubic spline interpolation on $S^{EXT}$ subject to the constraint that $S^{EXT}(|\mathbf{k}|) \to \alpha k^2$ as $|\mathbf{k}| \to 0$. With the splined form of $S^{EXT}(|\mathbf{k}|)$ in hand, we were able to numerically calculate the potential energy integration error, which is identified as the Chiesa correction.

For the kinetic energy correction, the originally published scheme requires the use of an optimized k-space Jastrow factor to capture the long-range electron correlations. As all of our Jastrow factors are short-ranged, the leading order VMC Chiesa scheme would yield no correction to the kinetic energy (at least to leading order). To get around this, we compare the difference in the potential energy corrections between using the extrapolated structure factor $S^{EXT}(\mathbf{k})$ and the mixed estimator $S^{DMC}(\mathbf{k})$. The difference here is associated to be the magnitude of the kinetic energy correction. This is because performing the Chiesa correction scheme with mixed estimates of $S^{DMC}(\mathbf{k})$ yields the leading order correction to the total energy, but the partitioning of the finite size contributions stemming from the potential and kinetic terms will not be correct. Using instead $S^{EXT}(\mathbf{k})$ gives the correct finite size correction to the potential energy. Since mixed and extrapolated estimates should yield the same total energy correction, the change in potential energy must be offset by a compensating change in the kinetic energy. Since the leading order VMC kinetic energy correction is zero on account of the use of short-ranged jastrows, the change in potential energy yields the entire kinetic energy correction.

We also tested the original kinetic energy correction scheme, specifically by independently optimizing a k-space jastrow which we added to our already optimized short-ranged Slater-Jastrow wavefunction. Fitting this to the RPA form, we obtained the kinetic energy correction as described by Chiesa et al.[2]. We found this to be indistinguishable from our previously described method.

### *4. 1/N Extrapolations*

For each unit cell and super cell calculation, we perform a linear fit on each quantity $X$ with respect to 1/N. In Table V, we list the finite size corrections to various quantities, which are of the following form:

$$\Delta X_N = X_\infty - X_N \tag{9}$$

$X_\infty$ represents the value of $X$ in the thermodynamic limit, and $X_N$ represents the value of $X$ in a unit cell with $N$ particles.

| WF | Method | $N$ | $\Delta E$ | $\Delta V$ | $\Delta T$ | $\Delta V_{ee}$ | $\Delta V_{ee}(MPC)$ | $\Delta V_{ei}$ |
|---|---|---|---|---|---|---|---|---|
| 1 | VMC | 64 | 0.012145(4) | 0.04460(9) | -0.03245(9) | 0.00544(1) | 0.00685(1) | 0.0391(1) |
| | DMC | 64 | 0.00803(1) | 0.0254(1) | -0.01740(9) | 0.00537(4) | 0.00618(3) | 0.0200(1) |
| | EXTR | 64 | – | 0.0063(2) | 0.0017(2) | 0.00530(7) | 0.00551(6) | 0.0009(2) |
| 2 | VMC | 64 | 0.01534(1) | 0.0388(3) | -0.0228(1) | 0.02775(5) | 0.00585(2) | 0.0111(1) |
| | RMC | 64 | 0.00816(3) | 0.0164(2) | -0.0072(2) | 0.01452(7) | 0.00557(5) | 0.0012(2) |
| | EXTR | 64 | – | -0.0074(4) | 0.0085(4) | 0.0014(1) | 0.00529(5) | -0.0087(4) |
| | PURE | 64 | – | 0.0069(9) | 0.0014(5) | 0.0066(2) | 0.00538(8) | 0.0005(7) |

TABLE V: Summary of finite size corrections taken from 1/N extrapolation data on wavefunctions #1 and #2. All units are in Ha/N. Single-particle kinetic energy corrections have been included.

| Method | $N$ | $\Delta E$ | $\Delta V$ | $\Delta T$ | $\Delta V_{ee}$ | $\Delta V_{ei}$ |
|---|---|---|---|---|---|---|
| SS | 64 | 0.00816(3) | 0.0069(9) | 0.0014(5) | 0.0066(2) | 0.0005(7) |
| KZK | 64 | 0.00682 | - | - | - | - |
| Chiesa | 64 | 0.00735 | 0.0059 | 0.00143 | 0.0059 | 0.000 |
| MPC | 64 | 0.00538(8) | 0.00538(8) | - | 0.00538(8) | - |

TABLE VI: Summary of finite size corrections from supercell (SS), KZK, Chiesa, and MPC. Wavefunction #1 was used for everything except the supercell calculations. Units are in Ha/N.

Note that the single-particle kinetic energy corrections have been included in the calculation of the unit cell.

### D. Results & Comparison

In Table VI, we compare all mentioned methods of finite size corrections against the RMC supercell calculations. What we find is that the Chiesa scheme described previously is the most accurate for not only the total energy, but also for the kinetic and potential energy corrections as well. It is within 0.81mHa ($27\sigma$, where $\sigma$ is the standard deviation) for the total energy estimate, 1mHa ($1\sigma$) for the potential energy, and 0.5mHa ($1\sigma$) for the kinetic energy. It is interesting to note that if one were to calculate the kinetic energy correction through fitting the k-space jastrow (which was included in the trial wavefunction #2 from the previous section) to the standard RPA form yields a kinetic energy correction of 1.7mHa/N, which is again within error bars.

The MPC correction does fairly well for correcting $V_{ee}$, however the error is 0.5mHa lower than the Chiesa correction. Additionally, one still needs to resort to another method to obtain the kinetic energy correction, typically through either the RPA or Chiesa scheme.

For estimates of the total energy, the KZK correction performs fairly well, although the error is noticeably higher: 1.3mHa for KZK as opposed to 0.8mHa for Chiesa.

Due to the possibility of cancellation of errors in our test sets, the most pressing question is how well our finite-size correction scheme works over a range of configurations. To this end, for $r_s = 1.10$ and $r_s = 1.34$, and for all helium concentrations, we grabbed the first two configurations in each test set and performed supercell calculations as described in the first part of this section. We then calculated the Chiesa and MPC corrections for all considered configurations. In Table VII, we show the average and mean absolute deviation of the finite size correction scheme relative to the supercell calculation.

Some comments here are in order. First, though the total finite size error is approximately 1 mHa/N, these errors will largely cancel (to within 0.23mHa/N) when considering differences between configurations. Secondly, though the MAD seems large (between 0.35 and 0.5 mHa/N), one should keep in mind that this is calculated across all considered helium concentrations at a given density. Deviations within a particular density and helium configuration are expected

| Density | Quantity | $\Delta E^{SS}$ | $\Delta E^{Ch}$ | $\Delta E^{Ch} - \Delta E^{SS}$ |
|---|---|---|---|---|
| 1.10 | Mean | 8.52 | 7.33 | -1.20 |
| 1.34 | Mean | 6.36 | 5.39 | -0.97 |
| 1.10 | MAD | 0.38 | 0.14 | 0.50 |
| 1.34 | MAD | 0.22 | 0.17 | 0.35 |

TABLE VII: Mean and mean absolute deviation (MAD) of the supercell energy correction ($\Delta E^{SS}$), Chiesa energy correction ($\Delta E^{Ch}$ ), and Chiesa correction error, all in mHa/N units. Note that we consider two densities: $r_s = 1.10$ and $r_s = 1.34$.

to be significantly smaller.

---


[1] C. Lin, F. Zong, and D. Ceperley, Physical Review E **64**, 016702 (2001), ISSN 1063-651X, URL `http://link.aps.org/doi/10.1103/PhysRevE.64.016702`.

[2] S. Chiesa, D. Ceperley, R. Martin, and M. Holzmann, Physical Review Letters **97**, 6 (2006), ISSN 0031-9007, URL `http://link.aps.org/doi/10.1103/PhysRevLett.97.076404`.

[3] S. Chiesa, D. Ceperley, and S. Zhang, Physical Review Letters **94**, 036404 (2005), ISSN 0031-9007, URL `http://link.aps.org/doi/10.1103/PhysRevLett.94.036404`.

[4] N. Troullier and J. L. Martins, Physical Review B **43**, 1993 (1991).

[5] H. Kwee, S. Zhang, and H. Krakauer, Phys. Rev. Lett. **100**, 126404 (2008), URL `http://link.aps.org/doi/10.1103/PhysRevLett.100.126404`.

[6] L. Fraser, W. Foulkes, G. Rajagopal, R. Needs, S. Kenny, and A. Williamson, Physical Review B **53**, 1814 (1996), ISSN 0163-1829, URL `http://link.aps.org/doi/10.1103/PhysRevB.53.1814`.

[7] N. Drummond, R. Needs, a. Sorouri, and W. Foulkes, Physical Review B **78**, 125106 (2008), ISSN 1098-0121, URL `http://link.aps.org/doi/10.1103/PhysRevB.78.125106`.
